# Supplementary material for: SEM-ROVER: Semantic Voxel-Guided Diffusion for Large-Scale Driving Scene Generation
Source: arXiv:2604.06113 source file (2026-04-07)
Supplement: Supplementary file 1 [file voxelfield_diff.tex]

\centering
\includegraphics[width=\linewidth]{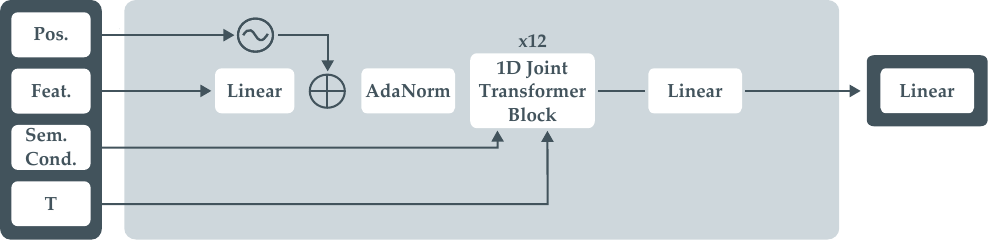}
